# Supplementary material for: Coordinated Multi-Agent Pathfinding for Drones and Trucks over Road Networks
Source: arXiv:2110.08802 source file (2022-02-10)
Supplement: Supplementary file 1 [file appendix.tex]

\appendix

\section*{Comparing on Capacity = 1}

The setting of 5 cars and 5 drones was the only one where the majority of 20 trials for ECBS did not time out due to too many conflicts ($> 1000$). The average distance for ECBS was $\SI{64.4}{\kilo\metre}$ and for PP was $\SI{65.3}{\kilo\metre}$. For plan time, the average for ECBS was $\SI{2.92}{\second}$ and that for PP was $\SI{2.51}{\second}$.
